# Supplementary material for: Assessing the persistence of chalcogen bonds in solution with neural network potentials
Source: arXiv:2201.04503 source file (2022-01-12)
Supplement: Supplementary file 1 [file AMOEBA_system.pdf]

```
##############################
##                          ##
##   Force Field Definition ##
##                          ##
##############################
```

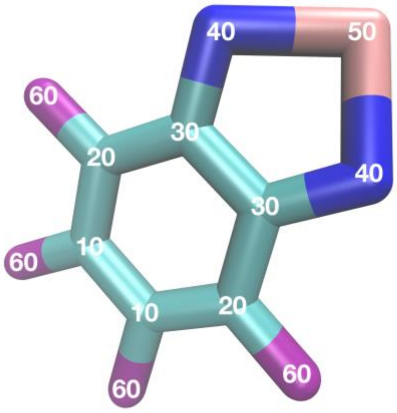


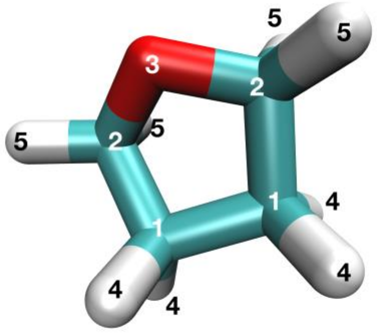


```
forcefield              AMOEBA-system

bond-cubic              -2.55
bond-quartic            3.793125
angle-cubic             -0.014
angle-quartic           0.000056
angle-pentic            -0.0000007
angle-sextic            0.000000022
opbendtype              ALLINGER
opbend-cubic            -0.014
opbend-quartic          0.000056
opbend-pentic           -0.0000007
opbend-sextic           0.000000022
torsionunit             0.5
vdwtype                 BUFFERED-14-7
radiusrule              CUBIC-MEAN
radiustype              R-MIN
radiussize              DIAMETER
epsilonrule             HHG
dielectric              1.0
polarization            MUTUAL
vdw-12-scale            0.0
vdw-13-scale            0.0
vdw-14-scale            1.0
vdw-15-scale            1.0
mpole-12-scale          0.0
mpole-13-scale          0.0
mpole-14-scale          0.4
mpole-15-scale          0.8
polar-12-scale          0.0
polar-13-scale          0.0
polar-14-scale          1.0
polar-15-scale          1.0
```

```
polar-12-intra          0.0
polar-13-intra          0.0
polar-14-intra          0.5
polar-15-intra          1.0
direct-11-scale         0.0
direct-12-scale         1.0
direct-13-scale         1.0
direct-14-scale         1.0
mutual-11-scale         1.0
mutual-12-scale         1.0
mutual-13-scale         1.0
mutual-14-scale         1.0

atom           1     1    C     "input              "        6    12.011    4
atom           2     2    C     "input              "        6    12.011    4
atom           3     3    O     "input              "        8    15.999    2
atom           4     4    H     "input              "        1     1.008    1
atom           5     5    H     "input              "        1     1.008    1
atom          10    10    C     "input              "        6    12.011    3
atom          20    20    C     "input              "        6    12.011    3
atom          30    30    C     "input              "        6    12.011    3
atom          40    40    N     "input              "        7    14.007    2
atom          50    50    Te    "input              "       24    51.996    2
atom          60    60    F     "input              "        9    18.998    1
atom          70    70    F     "input              "        9    18.998    1
atom         413    84    Cl-   "Chloride Ion Cl-"          17    35.453    0
atom         352    93    Na+   "Sodium Ion Na+"            11    22.990    0

vdw           1              3.820     0.1010
vdw           2              3.820     0.1010
vdw           3              3.405     0.1100
vdw           4              2.780     0.0260     0.91
vdw           5              2.780     0.0260     0.91
vdw          10              3.800     0.0890
vdw          20              3.800     0.0890
vdw          30              3.800     0.0890
vdw          40              3.710     0.1100
vdw          50              1.000     0.1000
vdw          60              3.220     0.1200
vdw          70              3.220     0.1200
vdw          84              4.1300    0.3400
vdw          93              2.9550    0.2800

bond          1    2         385.0     1.5276
bond          1    1         385.0     1.5300
bond          1    4         400.0     1.0939
bond          2    3         465.0     1.4308
bond          2    5         400.0     1.0961
bond         10   20         680.0     1.3767
bond         10   10         680.0     1.4195
bond         10   70         350.0     1.3329
bond         20   30         680.0     1.4211
bond         20   60         350.0     1.3320
bond         30   30         680.0     1.4540
bond         30   40         435.0     1.3597
bond         40   50         600.0     1.9537

angle         1    1    2    60.00     100.76
angle         2    1    4    38.00     111.57
angle         1    1    4    38.00     111.91
angle         4    1    4    34.50     108.91
angle         1    2    3    88.00     106.27
angle         1    2    5    38.00     111.86
angle         3    2    5    51.50     109.02
angle         5    2    5    34.50     108.72
angle         2    3    2    88.50     109.24
angle        10   10   20    60.00     121.20
angle        20   10   70    60.00     120.84
```

```
angle        10   10   70     60.00     117.96
angle        10   20   30     60.00     119.49
angle        10   20   60     60.00     120.28
angle        30   20   60     60.00     120.23
angle        20   30   30     60.00     119.32
angle        20   30   40     60.00     121.13
angle        30   30   40     60.00     119.56
angle        30   40   50     65.00     104.77
angle        40   50   40     65.00      91.35

strbnd        1    1    2     18.70      18.70
strbnd        2    1    4     18.70      11.50
strbnd        1    1    4     18.70      11.50
strbnd        1    2    3     18.70      18.70
strbnd        1    2    5     18.70      11.50
strbnd        3    2    5     18.70      11.50
strbnd        2    3    2     38.00      38.00
strbnd       10   10   20     18.70      18.70
strbnd       20   10   70     18.70      18.70
strbnd       10   10   70     18.70      18.70
strbnd       10   20   30     18.70      18.70
strbnd       10   20   60     18.70      18.70
strbnd       30   20   60     18.70      18.70
strbnd       20   30   30     18.70      18.70
strbnd       20   30   40     18.70      18.70
strbnd       30   30   40     18.70      18.70
strbnd       30   40   50     14.40      14.40
strbnd       40   50   40     38.00      38.00

opbend       20   10    0    0           14.40
opbend       10   10    0    0           14.40
opbend       70   10    0    0           14.40
opbend       30   20    0    0           14.40
opbend       60   20    0    0           14.40
opbend       30   30    0    0           14.40
opbend       40   30    0    0           14.40
opbend       20   30    0    0           14.40
opbend       10   20    0    0           14.40

torsion       1    1    2    3      -1.150 0.0 1   0.000 180.0 2   1.280 0.0 3
torsion       1    1    2    5       0.000 0.0 1   0.000 180.0 2   0.340 0.0 3
torsion       4    1    2    3       0.000 0.0 1   0.000 180.0 2   0.300 0.0 3
torsion       4    1    2    5       0.000 0.0 1   0.000 180.0 2   0.300 0.0 3
torsion       2    1    1    2       0.180 0.0 1   0.170 180.0 2   0.520 0.0 3
torsion       2    1    1    4       0.000 0.0 1   0.000 180.0 2   0.340 0.0 3
torsion       4    1    1    2       0.000 0.0 1   0.000 180.0 2   0.340 0.0 3
torsion       4    1    1    4       0.000 0.0 1   0.000 180.0 2   0.300 0.0 3
torsion       1    2    3    2       2.000 0.0 1  -1.500 180.0 2   0.890 0.0 3
torsion       5    2    3    2       0.000 0.0 1   0.000 180.0 2   0.710 0.0 3
torsion      10   10   20   30      -0.670 0.0 1   4.000 180.0 2   0.000 0.0 3
torsion      10   10   20   60       0.000 0.0 1   2.500 180.0 2   0.000 0.0 3
torsion      70   10   20   30       0.000 0.0 1   2.500 180.0 2   0.000 0.0 3
torsion      70   10   20   60       0.000 0.0 1   2.500 180.0 2   0.000 0.0 3
torsion      20   10   10   20      -0.670 0.0 1   4.000 180.0 2   0.000 0.0 3
torsion      20   10   10   70       0.000 0.0 1   2.500 180.0 2   0.000 0.0 3
torsion      70   10   10   20       0.000 0.0 1   2.500 180.0 2   0.000 0.0 3
torsion      70   10   10   70       0.000 0.0 1   2.500 180.0 2   0.000 0.0 3
torsion      10   20   30   30      -0.670 0.0 1   4.000 180.0 2   0.000 0.0 3
torsion      10   20   30   40       0.000 0.0 1   2.500 180.0 2   0.000 0.0 3
torsion      60   20   30   30       0.000 0.0 1   2.500 180.0 2   0.000 0.0 3
torsion      60   20   30   40       0.000 0.0 1   2.500 180.0 2   0.000 0.0 3
torsion      20   30   30   20      -0.670 0.0 1   4.000 180.0 2   0.000 0.0 3
torsion      20   30   30   40       0.000 0.0 1   2.500 180.0 2   0.000 0.0 3
torsion      40   30   30   20       0.000 0.0 1   2.500 180.0 2   0.000 0.0 3
torsion      40   30   30   40       0.000 0.0 1   2.500 180.0 2   0.000 0.0 3
torsion      20   30   40   50       0.000 0.0 1   1.000 180.0 2   0.500 0.0 3
torsion      30   30   40   50       0.000 0.0 1   1.000 180.0 2   0.500 0.0 3
torsion      30   40   50   40       0.000 0.0 1   1.000 180.0 2   0.500 0.0 3
```

```
multipole     1    2    1              -0.15250
                                        0.22916    0.00000    0.08287
                                        0.36179
                                        0.00000   -0.53306
                                       -0.23397    0.00000    0.17127
multipole     2    3    1               0.06230
                                        0.09017    0.00000    0.29616
                                       -0.11293
                                        0.00000   -0.46585
                                       -0.30087    0.00000    0.57878
multipole     3    2    2              -0.29900
                                        0.48544    0.00000    0.34478
                                        0.42574
                                        0.00000   -0.86401
                                       -0.01140    0.00000    0.43827
multipole     2    3    1               0.06230
                                        0.09017    0.00000    0.29616
                                       -0.11293
                                        0.00000   -0.46585
                                       -0.30087    0.00000    0.57878
multipole     1    2    1              -0.15250
                                        0.22916    0.00000    0.08287
                                        0.36179
                                        0.00000   -0.53306
                                       -0.23397    0.00000    0.17127
multipole     4    1    2               0.07973
                                        0.03204    0.00000   -0.06216
                                        0.04469
                                        0.00000   -0.04419
                                        0.05194    0.00000   -0.00050
multipole     5    2    3               0.04012
                                        0.01588    0.00000   -0.12279
                                        0.06167
                                        0.00000    0.05420
                                       -0.00900    0.00000   -0.11587
multipole     5    2    3               0.04012
                                        0.01588    0.00000   -0.12279
                                        0.06167
                                        0.00000    0.05420
                                       -0.00900    0.00000   -0.11587
multipole     4    1    2               0.07973
                                        0.03204    0.00000   -0.06216
                                        0.04469
                                        0.00000   -0.04419
                                        0.05194    0.00000   -0.00050
multipole    10   70   10               0.21514
                                        0.15317    0.00000    0.24065
                                       -1.03165
                                        0.00000   -0.66659
                                       -0.35231    0.00000    1.69824
multipole    20   60   10               0.21524
                                       -0.08475    0.00000    0.58651
                                       -0.37394
                                        0.00000   -0.23261
                                       -0.23134    0.00000    0.60655
multipole    30   40   20               0.16596
                                       -0.09750    0.00000    0.49990
                                       -0.59606
                                        0.00000    0.36888
                                       -0.04317    0.00000    0.22718
multipole    30   40   20               0.16596
                                       -0.09750    0.00000    0.49990
                                       -0.59606
                                        0.00000    0.36888
                                       -0.04317    0.00000    0.22718
multipole    20   60   10               0.21524
                                       -0.08475    0.00000    0.58651
```

```
                                               -0.37394
                                                0.00000   -0.23261
                                               -0.23134    0.00000    0.60655
multipole    10   70   10                       0.21514
                                                0.15317    0.00000    0.24065
                                               -1.03165
                                                0.00000   -0.66659
                                               -0.35231    0.00000    1.69824
multipole    40   50   30                      -0.69142
                                                0.00447    0.00000   -0.00077
                                               -0.49229
                                                0.00000    0.10902
                                               -0.09143    0.00000    0.38327
multipole    50  -40  -40                       0.85176
                                                0.00000    0.00000    0.61915
                                                2.06462
                                                0.00000   -2.15872
                                                0.00000    0.00000    0.09410
multipole    40   50   30                      -0.69142
                                                0.00447    0.00000   -0.00077
                                               -0.49229
                                                0.00000    0.10902
                                               -0.09143    0.00000    0.38327
multipole    60   20   10                      -0.16864
                                                0.01571    0.00000    0.22047
                                               -0.30553
                                                0.00000   -0.20614
                                                0.00559    0.00000    0.51167
multipole    60   20   10                      -0.16864
                                                0.01571    0.00000    0.22047
                                               -0.30553
                                                0.00000   -0.20614
                                                0.00559    0.00000    0.51167
multipole    70   10   10                      -0.16216
                                                0.00888    0.00000    0.26522
                                               -0.29244
                                                0.00000   -0.22485
                                               -0.00236    0.00000    0.51729
multipole    70   10   10                      -0.16216
                                                0.00888    0.00000    0.26522
                                               -0.29244
                                                0.00000   -0.22485
                                               -0.00236    0.00000    0.51729
multipole   413    0    0                      -1.00000
                                                0.00000    0.00000    0.00000
                                                0.00000
                                                0.00000    0.00000
                                                0.00000    0.00000    0.00000
multipole   352    0    0                       1.00000
                                                0.00000    0.00000    0.00000
                                                0.00000
                                                0.00000    0.00000
                                                0.00000    0.00000    0.00000

polarize            1         1.3340     0.3900      1    2    4
polarize            2         1.3340     0.3900      1    3    5
polarize            3         0.8370     0.3900      2
polarize            4         0.4960     0.3900      1
polarize            5         0.4960     0.3900      2
polarize           10         1.7500     0.3900     10    20    70
polarize           20         1.7500     0.3900     10    30    60
polarize           30         1.7500     0.3900     20    30    40
polarize           40         1.0730     0.3900     30    50
polarize           50         3.9000     0.3900     40
polarize           60         0.5070     0.3900     20
polarize           70         0.5070     0.3900     10
polarize          413         4.0000     0.3900
polarize          352         0.1200     0.3900
```
